# Supplementary material for: Proving LTL Properties of Bitvector Programs and Decompiled Binaries (Extended)
Source: arXiv:2105.05159 source file (2021-08-28)
Supplement: Supplementary file 1 [file dumping.tex]

\section{DUMPING GROUND - temporary holding}

% fist eval table draft
\begin{center}
%\begin{table}[!h]
  %% \begin{adjustwidth}           
    %% \centering
    %\caption{\label{tab:experiments} Bit-wise Abstraction for LTL.}
     \begin{adjustbox}{max width=0.9\textwidth,center}
     
\setlength{\tabcolsep}{0.2em}
         \begin{tabular}{|l|c|c|cl||ccr||}
            \hline
            \textbf{Benchmark} & \textbf{Gnd} &  \textbf{ Source} & \multicolumn{2}{c||}{\textbf {\ultimate}} & \multicolumn{3}{c||}{\textbf {BitAbs}} \\
            \textbf{Program} & \textbf{Expected} & \textbf{LOC} & Time(s) & Res. & Time(s) & Res. & Rules \\
            \hline
            \texttt{ and\_guard.c } & \OK & 13 &  & \UNK &  & \OK & \textbf{AND-0}, AND-1 \\
            \texttt{ and\_guard1.c } & \OK & 15 &  & \UNK &  & \OK & \textbf{AND-0}, AND-1 \\
            \texttt{ and\_guard2.c } & \OK & 20 &  & \UNK &  & \OK & \textbf{AND-0}, AND-1 \\
            %% \texttt{ and\_guard3.c } & \OK & 15 &  & \OK &  & \OK \\
            %% \texttt{ and\_guard4.c } & \OK & 14 &  & \UNK &  & \OK & \\
            %% \texttt{ and\_guard5.c } & \OK & 15 &  & \OK &  & \OK \\
            \texttt{ and\_loop.c } & \OK & 31 &  & \UNK &  & \OK & \textbf{AND}, AND-1, AND-0 \\
            \texttt{ and\_loop1.c } & \OK & 20 &  & \UNK &  & \OK & \textbf{AND-1}, AND-0 \\
            \texttt{ and\_stem.c } & \OK & 14 &  & \UNK &  & \OK & \textbf{AND-0}, AND-1 \\
            \texttt{ and\_stem1.c } & \OK & 18 &  & \UNK &  & \OK & \textbf{AND-0}, AND, AND-1 \\
            \texttt{ and\_stem2.c } & \OK & 18 &  & \UNK &  & \OK & \textbf{AND-0},AND, AND-1 \\
            \texttt{ com\_loop.c } & \OK & 23 &  & \UNK &  & \OK & \textbf{CPL-POS, CPL-NEG} \\
            \texttt{ com\_stem.c } & \OK & 18 &  & \UNK &  & \OK & \textbf{CPL-POS}, CPL-NEG \\
            \texttt{ or\_guard.c } & \OK & 14 &  & \UNK &  & \OK & \textbf{OR-1}, OR-0 \\
            \texttt{ or\_loop.c } & \OK & 15 &  & \UNK &  & \OK & \textbf{OR-1}, OR-0\\
            \texttt{ or\_loop1.c } & \OK & 24 &  & \UNK &  & \OK & \textbf{OR}, OR-1, OR-0 \\
            \texttt{ or\_loop2.c } & \OK & 24 &  & \UNK &  & \OK & \textbf{OR-0}, OR, OR-1 \\
            \texttt{ or\_stem.c } & \OK & 14 &  & \UNK &  & \OK & \textbf{OR-1}, OR, OR-0 \\
            \texttt{ xor\_guard.c } & \OK & 15 &  & \UNK &  & \OK & \textbf{XOR-EQ}, XOR-NEQ, XOR-0 \\
            \texttt{ xor\_loop.c } & \OK & 17 &  & \UNK &  & \OK & \textbf{XOR-NEQ}, XOR-EQ, XOR-0 \\
            \texttt{ xor\_stem.c } & \OK & 15 &  & \UNK &  & \OK & \textbf{XOR-EQ}, XOR-NEQ, XOR-0 \\
            \texttt{ xor\_stem1.c } & \OK & 16 &  & \UNK &  & \OK &\textbf{XOR-0}, XOR-EQ, XOR-NEQ \\
            \hline
        \end{tabular}
  \end{adjustbox}
  \vspace{-1em}
%\end{table}
\end{center}

% fist eval table draft
\begin{table}[h]
  %% \begin{adjustwidth}           
    %% \centering
    \caption{\label{tab:experiments:ltl-dec} LTL Verificaiton Task for De-compiled Code.}
     \begin{adjustbox}{max width=0.9\textwidth,center}
     
\setlength{\tabcolsep}{0.2em}
         \begin{tabular}{|l|c|l|cr||cr||}
            \hline
            \textbf{Benchmark} & \textbf{Property} &  \textbf{Expected} & \multicolumn{2}{c||}{\textbf {Vanilla}} & \multicolumn{2}{c||}{\textbf {BitAbs}} \\
             &   &  & Time(s) & Res. & Time(s) & Res.  \\
            \hline
            \texttt{PotentialMinimizeSEVPABug} & \OK & $\square ((x>0) \rightarrow \lozenge (y==0))$ & 2.0 & \UNK & 11.7 & \OK\\
            \texttt{PotentialMinimizeSEVPABug-false} & \NOK & $\square ((x<0) \rightarrow \lozenge (y==0))$ & 1.6 & \UNK & 2.0 & \NOK\\
            \texttt{someNonterminating} & \NOK & $\square (x>0)$ & 1.0 & \UNK & 1.4 & \NOK\\
            \texttt{simple3-false} & \NOK & $\lozenge (p==2)$ & 3.4 & \UNK & 3.9 & \NOK\\
            \texttt{simple3} & \OK & $\lozenge (p==1)$ & 1.1 & \OK & 1.4 & \OK\\
            \texttt{01-exsec2\_true-valid-ltl-false} & \NOK & $\lozenge(\square(x != 1))$ & 1.0 & \UNK & 16.1 & \NOK\\
            \texttt{01-exsec2\_true-valid-ltl} & \OK & $\lozenge(\square(x == 1))$ & 0.5 & \OK & 0.6 & \OK\\
            
       \hline 
        \end{tabular}
  \end{adjustbox}
  \vspace{-1em}
\end{table}

\red{FIND A HOME FOR THIS:}

Our abstraction (Section~\ref{sec:abstraction}) consists of two kinds of rules. First, \emph{conditional rewriting} rules let us conditionally replace bitwise operations with simpler expressions. For example, the \texttt{R-And-1} rule is below on the left:
\[
\infer{a \& b \leadsto a}{(a=0\vee a=1)\wedge b = 1}
\hspace{1in}
\infer{r\leq a\&b \Rightarrow r \leq a \wedge r \leq b}{a \geq 0 \wedge b \geq 0}
\]
With this rule, an instruction that assigns the result of $a\&b$ to a variable $x$ can
be replaced with an \texttt{if-then-else} which, under the condition that $(a=0\vee a=1)\wedge b = 1$, instead directly assigns $a$ to $x$ and, otherwise, havocs\red{more detail?} $x$.
We also provide \emph{weakening} rules such as the one above on the right. This rule lets us replace bitwise comparison $r \leq a\& b$ with a linear comparison $r \leq a \wedge r \leq b$ (again, under certain conditions).
By over-approximating bit-precise integers and operations on those integers with linear arithmetic relations (\eg~$<,\leq,\neq,$ etc), we later show this often enables verification tools to reason about LTL properties of lifted binaries.
We have implemented our \red{XX} rules in our tool \Tool{}.
For the \code{PotentialMinimizeSEVPABug.c} example above, our implementation used the following rules:
RS-POS, RS-NEG, AND-LOG, AND-1, XOR-EQ, XOR-NEQ. \red{cyrus update this if any implementation rules change}

In addition to enabling verification of decompiled binaries, our abstraction also enables verification of numerous bitwise programs that previously could not be verified, include \red{X} examples drawn from Sean Anderson's ``BitHacks'' repository\footnote{https://graphics.stanford.edu/~seander/bithacks.html}.

\red{FIND A HOME FOR THIS:}

%block_401159:                                     
  %29 = phi i64 [ %28, %block_401119 ], [ %55, %block_401159.backedge ]
  %30 = phi %struct.Memory* [ %25, %block_401119 ], [ %56,... %block_401159.backedge ]
  %31 = load i32, i32* bitcast (%x_type* @x to i32*)
  %32 = add i64 %29, 8
  %33 = icmp eq i32 %31, 0
  %34 = lshr i32 %31, 31
  %35 = xor i1 %33, true
  %36 = icmp eq i32 %34, 0
  %37 = and i1 %36, %35
  %38 = select i1 %37, i64 -44, i64 2
  %39 = add i64 %38, %32
%  br i1 ( ((x >> 31) == 0) && ((x == 0) ^ true) ), label %block_401135, label %block_401163
Above, the \code{if} statement on Line~\ref{ln:xpos} is a bitwise calculation equivalent to \code{x>0} and the \code{if} statement on Line~\ref{ln:xone} is equivalent to \code{x<=1}.
The variable \code{x} in the statement on Line~\ref{ln:xpos} is a signed integer but, 
%corresponds to the condition “x > 0” in the original source code, where “x” is an “signed integer”;
when the original source code is translated into binary code, type of \code{x} is stripped and thus, after decompilation, the type of \code{x} is unknown. To approximate, lifting procedures consider \code{x} (and all integers) to be unsigned.
% (McSema considers every integer unsigned)
Meanwhile, in the binary, the \emph{condition} \code{x>0} is compiled to be a \emph{signed} comparison.
Therefore, a lifting procedure (\eg~\mcsema) will create a signed comparison using the unsigned version of \code{x}. Roughly, the lifting process proceeds as:
\[\begin{array}{ll}
\code{(int)x > 0} 
&\leadsto \code{x != 0 \&\& x <= 0x7fffffff}\\ 
&\leadsto \code{x != 0 \&\& (x>>31) == 0}\\
&\leadsto \code{x != 0 \&\& (  ((x>>31) == 0) \^ 1)}
\end{array}\]
%; That means MeSema will need to run a signed comparison using the “unsigned version” of “x”; That means “(int)x > 0” ===> “x != 0 && x <= 0x7fffffff” ====> “x != 0 && (x>>31) == 0” ====> “x != 0 && (  ((x>>31) == 0) ^ 1)”
The decompilation process for Line~\ref{ln:xone} involves similar complexities.
The end result is that we are left with a multitude of 
bitwise operations, which are challenging for existing tools, which are more geared toward linear arithmetic reasoning.

With the target of liveness (LTL) properties we therefore introduce a novel abstraction over bitwise expressions/statements that (i) exploits bitwise paradigms common in lifted code and (ii) over-approximates bitwise expressions with linear equalities/inequalities, which are more amenable to verification tools that seek linear rank functions.
