# Supplementary material for: Proving LTL Properties of Bitvector Programs and Decompiled Binaries (Extended)
Source: arXiv:2105.05159 source file (2021-08-28)
Supplement: Supplementary file 2 [file lift.tex]

\section{Lifting to \IRde}
\label{sec:simplify}
%Re-engineering for Verification.
\todo{stack array issue in ultimate}

In this section we describe analyses and translations to
lift decompiled binaries into \IRde.

\red{update}
Unfortunately, although they emit LLVM IR or C programs, 
these resulting programs are out of reach for today's 
verification tools. Such tools will typically report 
false positives in the form of infeasible counterexamples 
(see Section~\ref{sec:eval}).

To facilitate the accessibility of binary verification, we 
leverage the widely-used IDA Pro~\cite{ferguson2008reverse} 
for disassembly and McSema~\cite{dinaburg2014mcsema} for de-compilation. 

Intuitively, the problem is that \emph{the de-compilation
by \mcsema\ strives for re-compilation, which is 
optimized for correctness and efficiency but less for verification}.
We now describe the major ways in which we re-engineer 
the de-compilation to make lifted code more amenable to verification.

\subsection{Removing verification-unrelated code and data} 

%whether the values of {\tt PATH} are in the 
%Consequently, this portion of \IRde is  independent of the particular program that is being simulated and can be excluded for the purposes of verification.
%. Excluding these pieces of code makes no difference to the verification results.
\red{less tooly}
\Tool\ analyzes McSema's output \IRde and decouples
the context-switch code from the code that simulates the 
original program. To this end, \Tool\ first locates the original 
{\tt main} function in the simulated code and then follows the 
control flow to extract statically reachable code. Further, the context-switch code also includes  program-independent functions 
that are registered to be executed before the {\tt main} or after 
the {\tt exit}. To avoid missing such functions in verification, 
we allocate calls to them at the begin or the end of the {\tt main} 
function, following the order these functions are 
registered to run in the original binary. 

\paragraph{Soundness of transformation.} Given binary program 
$P$, McSema creates \IRde to simulate every instruction in
$P$ and insert the context-switch code. Our transformation 
is essentially stripping the context-switch code, resulting 
in code semantically equivalent to $P$. Our transformation 
ensures soundness. \jun{Please correct this if wrong.}

\begin{figure}[!t]
\begin{minipage}{0.54\textwidth}
	\centering
	\textbf{Before Simplifying}
    \begin{lstlisting}[language=C,basicstyle=\scriptsize]
struct OC_State g_state;
int main(){
  struct OC_State *tmp = &g_state
  ...
  foo(tmp, 0, 0);
  ...
  return 0;
}
void foo(OC_State* tmp1, uint64_t tmp2, void* tmp3){
  struct OC_anon* tmp4;
  ...
  // field access via argument
  tmp4 = (&tmp1->field6);
  ...
  error(tmp1,tmp2,tmp3); // sim. args.
  ...
}
    \end{lstlisting}
\end{minipage}
\qquad
\begin{minipage}{0.42\textwidth}
	\centering
	\textbf{After Simplifying}
    \begin{lstlisting}[language=C,basicstyle=\scriptsize]
struct OC_State g_state;
struct OC_State* g_ptr 
  = &g_state;
int main(){
  ...
  foo();  // Arguments removed
  ...
  return 0;
}
void foo(){
  struct OC_anon* tmp4;
  ...
  // field access via global
  tmp4 = (g_ptr->field6); 
  ...
  error();  // Args. removed
  ...
}
    \end{lstlisting}
\end{minipage}
  \caption{Example showing our argument removal. In the {\tt main} function before our simplification, {\tt tmp}, which points to a global data structure {\tt g\_state}, is passed to the {\tt foo} function and its alias {\tt tmp1} is further passed to {\tt error}. After our simplification, all the arguments are removed, and the accesses to {\tt tmp} and {\tt tmp1} are fixed.}
  \label{fig:simplify}
\end{figure}

\subsection{Simplifying function arguments} 

In the absence of arguments, a procedural program begins to look and behave more like a \texttt{goto} program. Automata-based verification tools perform well on such parameter-less procedural programs, because calls and returns can be treated simply as edges in the automaton.

%The challenge is therefore how to make the procedures in 
For verification, \IRde should thus have as few arguments as possible, ideally removing all of them. Fortunately, it is easy: the first argument always points to the same global data structure and the other two arguments are not used. As such, \Tool\ eliminates all three arguments from every function call. We then create a pointer pointing to the global data struct
and replace all uses of the first argument with uses of our new pointer.
For example, as shown in Fig.~\ref{fig:simplify}, the output $\IRde'$ of \Tool\ replaces
\texttt{tmp1->field6} with \texttt{g\_ptr->field6}.

\paragraph{Soundness of transformation.} Our transformation 
removes two unused arguments and replaces a pointer with its 
alias. The produced code is semantically equivalent
to the original code. Our transformation ensures soundness.

\subsection{Flattening nested structures}

Many of the grouped constructs are functionally independent and hence the complex nesting is not necessary to maintain the original semantics. \Tool\ therefore flattens the data structures, producing a functionally equivalent $\IRde'$.  \Tool\ creates individual variables for all the innermost and separable fields. We then must translate accesses to these nested structures. To this end, we rely on use-define reasoning to identify all the accesses to a flattened field and perform corrections on-demand. For instance, for the aforementioned {\tt state->}{\tt general\_registers.}{\tt register13.}{\tt union.}{\tt uint64cell}, we allocate a new global variable {\tt register13} with the same type of {\tt uint64cell} and re-locate all the original accesses to {\tt register13}. 

\paragraph{Soundness of transformation.} Our use-define approach 
is sound because McSema never splits an access 
(\eg\ first access {\tt state->}{\tt general\_}{\tt registers} 
and then access {\tt register13.}{\tt union.}{\tt uint64cell}).
That is, our transformation is equivalent to replacing the symbol 
names of variables, which ensures the soundness.

\subsection{Refining type-casting}

%We present such an example in Table~\ref{tab:fixtype}.

\Tool\ revokes such short-cuts in type-casting, making the dereference more explicit as shown on the right.
%Table~\ref{tab:fixtype} also demonstrates the idea of our strategy. 

McSema also often brings redundant type-casting. For instance, 
it can create operations like {\tt *((int*)(\&p))} even if 
{\tt p} has the type of {\tt int}. \Tool\ strips redundant
type-casting, in a way such as changing {\tt *((int*)(\&p))} 
to {\tt *(\&p)} (and further to {\tt p}).

\paragraph{Soundness of transformation.} Our transformation 
replaces ``implicit'' typecasting with the ``explicit'' version
or removes redundant type-casting. It brings no change to 
the semantics and thus, ensures the soundness.

%After our lifting process, we use DG project ~\cite{chalupa_mchalupadg_online} to slice our de-compiled code, the slicing starts with a selected criteria, it slices out all the reachable nodes from this criteria in its main bytecode. Slicing can help reduce the size of program to be verified, improves the efficiency of verification task~\cite{chalupa_dg_nodate}. The slicing criteria can either be a function call, a global variable in a certain location, or a combination of multiple criteria pairs. In our implementation for the $LTL$ verification task, we choose the global variables in our $LTL$ properties as slicing criteria pairs. 
