# Supplementary material for: Proving LTL Properties of Bitvector Programs and Decompiled Binaries (Extended)
Source: arXiv:2105.05159 source file (2021-08-28)
Supplement: Supplementary file 3 [file decompile.tex]

\section{Problems from Decompliation}
Decompile binary to more high level code, but many ops are implemented with bitwise operations.
